# Supplementary material for: Cost-efficient Data Acquisition on Online Data Marketplaces for Correlation Analysis
Source: arXiv:1808.09545 source file (2018-08-28)
Supplement: Supplementary file 1 [file appendix.tex]

\appendix

\nop{
\section{Proof of Theorem 4.1}

First, we present some lemmas to show an important property of the partition-based information entropy under the existence of FDs. 
\begin{lemma}
\label{lm:entropy_p2}
Given any exact functional dependency $X\rightarrow Y$, it must be true that $H(Y)\leq H(X)$.
\end{lemma}
\noindent{\bf Proof.} Consider the FD $X\rightarrow Y$. It must be true that for any $eq_Y^i \in \pi_Y$, there exist a set of equivalence classes $\{eq_X^j\}\subseteq \pi_X$ such that: (1) $eq_X^j\subseteq eq_Y^i$, and (2) $\bigcup eq_X^j = eq_Y^i$ \cite{huhtala1999tane}. 
In other words, for any $eq_Y^i\in \pi_Y$, there must exist a set of equivalence classes $\{eq_X^j\}\subseteq \pi_X$ such that: (1) $P(eq_X^j)\leq P(eq_Y^i)$, and (2) $\sum P(eq_X^j) = P(eq_Y^i)$. 
Therefore, for any $eq_Y^i$, it must be true that $-P(eq_Y^i)\log_2 P(eq_Y^i) \leq -\sum P(eq_X^j)\log_2 P(eq_X^j)$. As a result, $H(Y)\leq H(X)$.

\begin{lemma}
\label{lm:entropy_p1}
Given any exact functional dependency $X\rightarrow Y$, it must be true that $H(XY) = H(X)$.
\end{lemma}
\noindent{\bf Proof.}
The proof is straightforward, as $X\rightarrow Y$ dictates that $\pi_{XY}=\pi_{X}$ \cite{huhtala1999tane}. Naturally $X$ and $XY$ have the same entropy.

One important property of functional dependency is the transitivity, i.e., if $X\rightarrow Y$ and $Y\rightarrow Z$, it must be true that $X\rightarrow Z$. Next, we use a lemma to show the pricing function in the existence of transitive FDs.
\begin{lemma}
\label{lm:entropy_p2}
Given two exact functional dependencies $X\rightarrow Y$ and $Y\rightarrow Z$, it must be true that $H(XYZ)=H(X)$.
\end{lemma}
\noindent{\bf Proof.}
The proof is straightforward, as we can infer that $X\rightarrow YZ$. By leveraging Lemma \ref{lm:entropy_p1}, it is easy to see that $H(XYZ)=H(X)$.

\noindent{\bf Proof. of Theorem \ref{theorem:entropy_af}}
The definition of the arbitrage-free condition relies on the notion of {\em determinacy} \cite{koutris2015query}. 
\begin{definition}
\label{df:determinacy}
Given two queries $Q_1$ and $Q_2$, we say $Q_2$ determines $Q_1$, denoted as $D\vdash Q_2 \rightarrow Q_1$, if for any instance $D'$, $Q_2(D)=Q_2(D')$ implies $Q_1(D)=Q_1(D')$.
\end{definition}

We use the following lemma to show how FDs impact determinacy. 
\begin{lemma}
\label{th:equiv}
Given a FD $F: X\rightarrow Y$, and two projection queries $Q_1$ and $Q_2$, where $Q_1$ and $Q_2$ applies projection on attributes $Y$ and $X$ (right-hand-side and left-hand-side of $F$) respectively, it must true that $D\vdash Q_2 \rightarrow Q_1$.
\end{lemma}
\noindent{\bf Proof.} Due to the FD $X\rightarrow Y$, if for any instance $D'$, $Q_2(D)=Q_2(D')$, it must be true that $Q_1(D)=Q_1(D')$. Then the theorem follows.

Based on Definition \ref{df:arbitrage-free} and Lemma \ref{th:equiv}, we have the following lemma that shows the sufficient condition of the arbitrage-free projection query based pricing function. 
\begin{lemma}
\label{th:affd}
A pricing function $p()$ is arbitrage-free for the vertical pricing model if for any FD $X\rightarrow Y$, $p(Y)\leq p(X)$.
\end{lemma}
We omit the proof of Theorem \ref{th:affd} due to the straightforwardness. 

Based on Lemma \ref{lm:entropy_p2}, for any FD $X\rightarrow Y$, $H(Y)\leq H(X)$. Then if the pricing function $p()$ is non-decreasing on $H(X)$, if must true that $p(Y)\leq p(X)$. Therefore, it is arbitrage-free by following Theorem \ref{th:affd}. \qed
}

\nop{
\section{Proof of Theorem 5.1}

Given two data instances $D_i$ and $D_j$, the attribute set $S$ of $D_i$, and two attribute sets $S_1$ and $S_2$ of $D_j$. Let $\mathcal{L}$ be the attribute set lattice of $D_j$, and $v_i$ and $v_j$ be the corresponding vertices of $S_1$ and $S_2$ in $\mathcal{L}$ respectively. We consider the following cases, based on the structure relationship between $v_1$ and $v_2$. We use $\mathcal{D}_1$ and $\mathcal{D}_2$ to denote $\{D_i, \pi_{S_1}(D_j)\}$ and $\{D_i, \pi_{S_2}(D_j)\}$ respectively. In other words, $\mathcal{D}_1$ ($\mathcal{D}_2$, resp.) denotes the join between $D_i$ and $\pi_{S_1}(D_j)$ ($\pi_{S_2}(D_j)$, resp.)

\begin{itemize}

\item Case 1: When $v_2$ is a sibling of $v_1$ (i.e. $v_1$ and $v_2$ are at the same level of $\mathcal{L}$)

\begin{itemize}

\item Case 1.1.: $S_1\cap S_2 \neq \emptyset$, and $S\cap S_1 = S \cap S_2$ (i.e., $\pi_{S} (D_i)$ joins with $\pi_{S_1} (D_j)$ on the same attribute set as $\pi_{S_2} (D_j)$). 
For this case, $JS({\mathcal{D}_1}) = JS({\mathcal{D}_2})$. On the hand hand, if $Q(\{\pi_{S_1}(D_j)\})\geq Q(\{\pi_{S_2}(D_j))$, then $Q(\mathcal{D}_1) \geq Q(\mathcal{D}_2)$, and vice versa, where $Q()$ is the qualify function defined in Formula \ref{def:qmsmfd} \Boxiang{I think this may not hold under the new definition of quality. The quality of $\mathcal{D}$ is defined on the join result, rather than the sum of quality on individual instances.}. This is because the error records that can(not) be joined will be included (excluded) in the join results. Therefore, if $Q(\{\pi_{S_1}(D_j)\})\geq Q(\{\pi_{S_2}(D_j))$, then $F(\mathcal{D}_1) \geq F(\mathcal{D}_2)$.  
Consider an example that two instances $D_i(A, B)$ and $D_j(A, C, D)$. Assume $S= \{A, B\}$, $S_1 =\{A, C\}$ and $S_2 = \{A, D\}$. We prefer to pick $\pi_{S_1}(D_j)$ to be joined with $D_i$ if the quality of $\pi_{S_1} (D_j)$ is better than $\pi_{S_2} (D_j)$. 

\item Case 1.2.: $S_1\cap S_2 \neq \emptyset$, and $S\cap S_1 \neq S \cap S_2$ (i.e., $\pi_{S} (D_i)$ joins with $\pi_{S_1} (D_j)$ on different attribute set as $\pi_{S_2} (D_j)$). 
As an example, consider two instances $D_i (A, B)$ and $D_j (A, B, D)$. Assume $S= \{A, B\}$, $S_1 =\{A, D\}$ and $S_2 = \{B, D\}$. In this case, $D_i$ joins with $\pi_{S_1}(D_j)$ on $A$, while with $\pi_{S_2} (D_j)$ on $B$. Due to different join attribute sets, it is difficult to infer the relationship between quality and join strength. 

\item Case 1.3: $S_1\cap S_2 = \emptyset$, and $S_1\cap S \neq S_2 \cap S$. This case is similar to Case 1.2. Different join attributes lead to no relationship between quality and join strength. 

\item Case 1.4: $S_1\cap S_2 = \emptyset$, and $S_1\cap S = S_2 \cap S$. This case will never happen as $S_1\cap S = S_2 \cap S$ infers that $S_1\cap S_2 \neq \emptyset$. 

\end{itemize}

\item Case 2: When $v_2$ is a parent/ancestor $v_1$ in $\mathcal{L}$ (i.e., $v_1$ and $v_2$ are on the same path, while $v_2$ is higher in $\mathcal{L}$). 

\begin{itemize}

\item Case 2.1: $S_1\cap S = S_2 \cap S$ (i.e., $\pi_{S} (D_i)$ joins with $\pi_{S_1} (D_j)$ on the same attribute set as $\pi_{S_2} (D_j)$). 
For this case, apparently, $JS({\mathcal{D}_1})$ = $JS({\mathcal{D}_2})$, due to the same join attributes. On the other hand,  
it always holds that $Q(\{D_i, \pi_{S_1}(D_j)\})\leq Q(\{D_i, \pi_{S_2}(D_j)\})$, since $D_i \bowtie \pi_{S_2}(D_j)$ has the same records as $D_i \bowtie \pi_{S_1}(D_j)$ but fewer attributes. Therefore, $F(\mathcal{D}_1)\leq F(\mathcal{D}_2)$. As an example, consider two instances $D_i(A, B)$ and $D_j(A, C, D)$. Assume $S= \{A, B\}$, $S_1 =\{A, C, D\}$ and $S_2 = \{A, C\}$.  We prefer to pick $\pi_{S_2} (D_j)$ to be joined with $D_i$ due to its better quality (and thus better value on objective function).

\item Case 2.2: $S_1\cap S \neq S_2 \cap S$ (i.e., $\pi_{S} (D_i)$ joins with $\pi_{S_1} (D_j)$ on different attribute set from $\pi_{S_2} (D_j)$). For this case, since $S_2$ is a parent of $S_1$, it must be true that $(S_2\cap S) \subset (S_1 \cap S)$. According to Property \ref{property:mono}, $JS({\mathcal{D}_1})\geq JS({\mathcal{D}_1})$. 
However, there is no relationship between $Q(\mathcal{D}_1)$ and $Q(\mathcal{D}_2)$. 
Consider an example that two instances $D_i(A, B, D)$ and $D_j(A, B, C, D)$. Assume $S= \{A, B, D\}$, $S_1 =\{A, B, C, D\}$ and $S_2 = \{A, B, C\}$.    
It is true that $\pi_{S_2}(D_j)$ has better quality than $\pi_{S_1}(D_j)$. But $S_1$ requires join of more attributes, which may lead to more error records excluded in the join result. 
%because the number of error tuples in $S_2$ cannot be less than that of $S_1$, and the size of join result of $S$, $S_2$ cannot be greater than that of $S$, $S_1$, we have $error_{SS_1}\le error_{SS_2}$. 
\end{itemize}

\item Case 3: When $v_1$ and $v_2$ are not either at the same path nor at the same level in $\mathcal{L}$. For this case, as $S_1$ and $S_2$ have no relationship, it is diffilcut to infer the relationship of $\pi_{S_1}(D_j)$ and $\pi_{S_2}(D_j)$. 

\end{itemize}

Let $v_{opt}$ be the best candidate. We discuss the following cases:
\begin{itemize}
\item For all ancestors of $v_{opt}$ that have the same join attributes as $v_{opt}$, they cannot win $v_{opt}$ because... (discuss two cases, $v_{opt}$ is a 2-attribute set, and it is not).
\item  For all ancestors of $v_{opt}$ that have different join attributes as $v_{opt}$, they cannot win $v_{opt}$ because...(discuss two cases, $v_{opt}$ is a 2-attribute set, and it is not).
\item For all siblings of $v_{opt}$ that have the same join attributes as $v_{opt}$, they cannot win $v_{opt}$, due to Case 1.1.  
\item For all siblings of $v_{opt}$ that have different join attributes as $v_{opt}$, they cannot win $v_{opt}$ because:
\item For all descendants of $v_{opt}$ that have the same join attributes as $v_{opt}$, they cannot win $v_{opt}$ because...
\item For all descendants of $v_{opt}$ that have different join attributes as $v_{opt}$, they cannot win $v_{opt}$ because...
\item For all remaining vertices that are neither on the same path as $v_{opt}$ or a sibling of $v_{opt}$, they cannot win $v_{opt}$ because...
\end{itemize}

Let $S_{opt}$ be the best candidate. Any attribute set in $D_j$ that can be joined with $D_i$ must be in the format of $Y\cup Z$, where $Y\subseteq X$, $Y\neq \emptyset$, $Z\subseteq D_j\setminus X$, and $Z\neq \emptyset$.
It is easy to see that for any such attribute set $S''$, there must exist an attribute set $S'\in SA(D_j)$ such that $S''\cap S=S'\cap S$, and $S'\subseteq S''$.
According to Case 2.1, it is guaranteed that $F(\{D_i, \pi_{S'}(D_j)\geq F(\{D_i, \pi_{S''}(D_j)\})\})$.
Also, we are sure that for any $S'\in SA(D_j)$,  $F(\{D_i, \pi_{S_{opt}}(D_j)\geq F(\{D_i, \pi_{S'}(D_j)\})\})$. 
Therefore, for any attribute set $S''$ in $D_j$ that can be joined with $D_i$, it must be true that $F(\{D_i, \pi_{S_{opt}}(D_j)\geq F(\{D_i, \pi_{S''}(D_j)\})\})$. In other words, $S_{opt}$ yields the best objective value.

Intuitively, for each path in the lattice, Case 2.1 ensures that picking the 2-attribute sets always deliver the better value of object function compared with k-attribute sets where $k>2$. Case 1.1 ensures that picking the 2-attribute of the best quality for join will always lead to the best value of the object function. 
}

\section{Proof of Theorem 3.1}
\begin{proof}
Let $X$ and $Y$ be the join attribute in $D_1$ and $D_2$ respectively. Let $V$ be the set of unique values in $X$ and $Y$. 

According to the definition of join informativeness, we have 
\begin{equation*}
JI(D_1, D_2) = \frac{H(D_1.X, D_2.Y)-I(D_1.X, D_2.Y)}{H(D_1.X, D_2.Y)},
\end{equation*}
where $H(D_1.X, D_2.Y)=-\sum_{v\in V}p(v,v)\log p(v,v)$, and $I(D_1.X, D_2.Y)=\sum_{v]\in V} p(v,v)\log \frac{p(v,v)}{p_X(v)p_Y(v)}$.

Let $F(v_1,v_2)$ denote the frequency of $(v_1,v_2)$ in the outer join result between $D_1$ and $D_2$. We have 
\begin{equation*}
F(v_1,v_2)=
\begin{cases}
f_X(v_1)f_Y(v_2) & \text{ if } v_1\in X, v_2\in Y \text{ and } v_1=v_2 \\
f_X(v_1) & \text{ if } v_1\in X, v_1\not\in Y \\
f_Y(v_2) & \text{ if } v_2\not\in X, v_2\in Y
\end{cases}
\end{equation*}

The size of the outer join result is 
\begin{equation*}
|J| = \sum_{v\in X\cap Y} f_X(v)f_Y(v) + \sum_{v\not\in Y} f_X(v) + \sum_{v\not\in X} f_Y(v).
\end{equation*}

So the probability of $(v_1, v_2)$ in the outer join result is 
\begin{equation*}
p(v_1,v_2) = \frac{F(v_1, v_2)}{|J|}=
\begin{cases}
\frac{f_X(v_1)f_Y(v_2)}{\sum_{v\in X\cap Y} f_X(v)f_Y(v) + \sum_{v\not\in Y} f_X(v) + \sum_{v\not\in X} f_Y(v)} & \text{ if } v_1\in X, v_2\in Y \text{ and } v_1=v_2 \\
\frac{f_X(v_1)}{\sum_{v\in X\cap Y} f_X(v)f_Y(v) + \sum_{v\not\in Y} f_X(v) + \sum_{v\not\in X} f_Y(v)} & \text{ if } v_1\in X, v_1\not\in Y \\
\frac{f_Y(v_2)}{\sum_{v\in X\cap Y} f_X(v)f_Y(v) + \sum_{v\not\in Y} f_X(v) + \sum_{v\not\in X} f_Y(v)} \text{ if } v_2\not\in X, v_2\in Y
\end{cases}
\end{equation*}

For any value $v$, its frequency in $X$ after the outer join is
\begin{equation*}
F_X(v) = 
\begin{cases}
F(v,v)=f_X(v)f_Y(v) & \text{ if } v\in X, v\in Y \\
f_X(v) & \text{ if } v\in X, v\not\in Y \\
f_X(NULL)=\sum_{v\not\in X} f_Y(v) & \text{ if } v\not\in X, v\in Y  
\end{cases}
\end{equation*}
Straightforwardly, we have $|X|=|J|$, and $|Y|=|J|$. Thus, the probability 
\begin{equation*}
p_X(v) = 
\begin{cases}
\frac{f_X(v)f_Y(v)}{|J|} & \text{ if } v\in X, v\in Y\\
\frac{f_X(v)}{|J|} & \text{ if } v\in X, v\not\in Y \\
\frac{\sum_{v\not\in X} f_Y(v)}{|J|} & \text{ if } v\not\in X, v\in Y
\end{cases}
\end{equation*}

Let $p$ be the sampling probability for both $S_1$ and $S_2$. 
For any $(v_1, v_2)$, if $v_1\in X$, $v_2\in Y$ and $v_1=v_2$, the probability that $(v_1, v_2)$ is present in the outer join $J'$ of $S_1$ and $S_2$ is $p$, i.e., $h(v_1)=h(v_2)\leq p$. If $v_1\in X$, and $v_2\not\in Y$, then $(v_1, NULL)$ is present in $J'$ if $h(v_1)\leq p$. Hence, we have
\begin{equation*}
E(F'(v_1,v_2))=
\begin{cases}
p\times f_X(v_1)f_Y(v_2) & \text{ if } v_1\in X, v_2\in Y \text{ and } v_1=v_2 \\
p\times f_X(v_1) & \text{ if } v_1\in X, v_1\not\in Y \\
p\times f_Y(v_2) & \text{ if } v_2\not\in X, v_2\in Y
\end{cases}
\end{equation*}
Thus, we have $E(|J'|)=p|J|$. Hence, we have $E(p'(v_1,v_2))=\frac{E(F'(v_1,v_2))}{E(|J'|)}=p(v_1, v_2)$.
Similarly, we have 
\begin{equation*}
E(F_X'(v)) = 
\begin{cases}
p\times f_X(v)f_Y(v) & \text{ if } v\in X, v\in Y\\
p\times f_X(v) & \text{ if } v\in X, v\not\in Y \\
p\times \sum_{v\not\in X} f_Y(v) & \text{ if } v\not\in X, v\in Y
\end{cases}
\end{equation*}
It is easy to see that $E(p'_X(v))=p_X(v)$ and $E(p'_Y(v))=p_Y(v)$. 

Therefore, we can conclude that $E(JI(S_1, S_2))=JI(D_1, D_2)$
\end{proof}

\section{Proof of Theorem 3.2}
\begin{proof}
First, we prove that $E(CORR_{S_1\Join S_2}(\mathcal{A_S},\mathcal{A_T}))=CORR_{D_1\Join D_2}(\mathcal{A_S},\mathcal{A_T})$ and $E(Q(S_1\Join S_2))=Q(D_1\Join D_2)$.
Without loss of generality, we assume that $\mathcal{A_S}=\{X\}$ and $\mathcal{A_T}=\{Y\}$.
Let $x$ and $y$ be two attribute values of $X$ and $Y$. The pair $(x,y)$ exists in the join result $T_1\Join T_2$ if there exists an attribute value $v$ of $J$ s.t. there is a tuple $t_i\in T_1$ with $t_i[X]=x$ and $t_i[J]=v$, and a tuple $t_j\in T_2$ with $t_j[J]=v$ and $t_j[Y]=y$. Hence, the size of the join result is 
\[
|T_1\Join T_2|=\sum_{v\in J} F_1(v)F_2(v),
\] 
where $F_1(v)$ and $F_2(v)$ denotes the frequency of $v$ in $T_1$ and $T_2$ respectively.
For any $x\in X$, its probability in $T_1\Join T_2$ is 
\[
p(x)=\frac{\sum_{v\in J}\sum_{y\in Y} F_1(x,v)F_2(v,y)}{|T_1\Join T_2|}.
\]
And the probability of the pair $(x,y)$ in the join result is 
\[
p(x,y)=\frac{\sum_{v\in J} F_1(x,v)F_2(v,y)}{|T_1\Join T_2|}.
\]

However, the pair $(x,y)$ exists in the join of samples if there exists a value $v$ of $J$ s.t. the pair $(x,v)$ exists in $T_1$, $(v,y)$ exists in $T_2$, and $h(v)\leq p_{min}$, where $p_{min}=min\{p_1,p_2\}$, and $p_1$ and $p_2$ are the probability to draw samples from $T_1$ and $T_2$ respectively.
Hence, the expected join size of samples is 
\begin{equation}
\label{eq:join}
E(|S_1\Join S_2|)=\sum_{v\in J} p_{min}F_1(v)F_2(v)=p_{min}|T_1\Join T_2|.
\end{equation}
For any value $x$, its frequency in $S_1\Join S_2$ is 
\begin{equation}
F'(x)=\sum_{v\in V}
\begin{cases}
F_1(x,v)\sum_{y\in Y} F_2(v,y) & \text{if } h(v)\leq p_{min} \\
0 & \text{otherwise}
\end{cases}
\end{equation}
Thus, the expected frequency of $x$ in $S_1\Join S_2$ is 
\begin{equation}
\label{eq:fx}
E(F'(x))=\sum_{v\in J} p_{min} F_1(x,v) \sum_{y\in Y} F_2(v, y)=p_{min} F(x).
\end{equation}
As a consequence, the expected probability of $x$ in $S_1\Join S_2$ is 
\[
E(p'(x))=\frac{E(F'(x))}{E(|S_1\Join S_2|)}=p(x).
\]
Similarly, we have 
\[
E(p'(x,y))=p(x,y).
\]
According to the definition of correlation, the expected correlation of $X$ and $Y$ over $S_1\Join S_2$ is 
\begin{equation*}
\begin{split}
E(CORR_{S_1\Join S_2} (X,Y)) &= E(H'(X)) - E(H'(X|Y)) \\
& = -\sum_{x\in X} E(p'(x))\log E(p'(x)) + \sum_{(x,y)\in (X,Y)} E(p'(x,y))\log \frac{E(p'(x))}{E(p'(x,y))} \\
&= -\sum_{x\in X} p(x)\log p(x) + \sum_{(x,y\in (X,Y))} p(x,y) \log \frac{p(x)}{p(x,y)} \\
&= CORR_{T_1\Join T_2}(X,Y).
\end{split}
\end{equation*}

In order to prove that $E(Q(S_1\Join S_2))=E(Q(T_1\Join T_2))$, we assume there only exists a single AFD $X\rightarrow Y$ and a single equivalence class $eq_x\in \pi_{X}$ for the sake of simplicity. Let $eq_{xy}$ be the correct equivalence class for $eq_x$ in $T_1\Join T_2$. 
Based on the definition of quality, we have $Q(T_1\Join T_2)=p(x,y)$.
According to 
Equation \ref{eq:join} and \ref{eq:fx}, we have $E(p'(x,y))=p(x,y)$, where $p'(x,y)$ is the probability of $(x,y)$ in $S_1\Join S_2$. Therefore, we have 
\begin{equation*}
E(Q(S_1\Join S_2))=E(p'(x,y))=p(x,y)=Q(T_1\Join T_2).
\end{equation*}

Next, we prove that $E(CORR_{S_{1,2}'\Join S_3}(X,Y))=CORR_{T_1\Join T_2 \Join T_3}(X,Y)$, and $E(Q({S_{1,2}'\Join S_3}))=Q(T_1\Join T_2 \Join T_3)$.
Let $p_1$, $p_2$ and $p_3$ be the probability to draw samples from $T_1$, $T_2$ and $T_3$ respectively. Also, let $p_{1,2}$ denote the probability to draw samples from $S_1\Join S_2$. Suppose the join attribute between $T_1$ and $T_2$ is $U$, and the join attribute between $T_2$ and $T_3$ is $V$.

 For any $(x, u, v, y)$ that exists in $T_1\Join T_2 \Join T3$, it also resides in $S_{1,2}'\Join S_3$ if $h(u)\leq p_{min}^1=min\{p_1,p_2\}$, $g(v)\leq p_{min}^2=min\{p_2,p_3\}$, and $f(v)\leq p_{min}^3=min\{p_{1,2},p_3\}$, where $h$, $g$ and $f$ are the hash functions to draw samples. Following the above proof, we can infer that $E(p'(x))=p(x)$ and $E(p'(x,y))=p(x,y)$.
Therefore, it is natural that $E(CORR_{S_{1,2}'\Join S_3}(X,Y))=CORR_{T_1\Join T_2 \Join T3}(X,Y)$, and $E(Q({S_{1,2}'\Join S_3}))=Q(T_1\Join T_2 \Join T_3)$.
\end{proof}

\section{Proof of Theorem 4.1}
First, we prove that the correlation function $CORR(X,Y)$ is submodular. 
A function $f: 2^V \rightarrow \mathbb{R}$ is submodular if for all $X\subset Y\subseteq V$ and for all $z\not\in Y$, $f(X\cup \{z\})-f(X)\geq f(Y\cup \{z\}) + f(Y)$.
According to the definition of correlation (Section \ref{sc:corr}), we have 
\[CORR(X, V\setminus X)=H(X)+H(V\setminus X)-H(V),\]
and
\begin{multline}
CORR(X\cup \{z\}, V\setminus (X\cup \{z\}))-CORR(X, V\setminus X) \\
= H(X\cup \{z\})+H(V\setminus (X\cup \{z\}))-H(X)-H(V\setminus X) \\
= (H(X\cup \{z\})-H(X))+H(V\setminus (X\cup \{z\})-H(V\setminus X)).
\end{multline}

Similarly, we have 
\begin{multline}
CORR(Y\cup \{z\}, V\setminus (Y\cup \{z\}))-CORR(Y, V\setminus Y)\\
=(H(Y\cup \{z\})-H(Y))+H(V\setminus (Y\cup \{z\})-H(V\setminus Y)).
\end{multline}

Because 
$H(X\cup \{z\})-H(X)\geq H(Y\cup \{z\})-H(Y)$ and $H(V\setminus Y)-H(V\setminus (Y\cup \{z\}))\geq H(V\setminus X)-H(V\setminus (X\cup \{z\}))$, we can infer that 
\begin{multline}
CORR(X\cup \{z\}, V\setminus (X\cup \{z\}))-CORR(X, V\setminus X) \\
\geq CORR(Y\cup \{z\}, V\setminus (Y\cup \{z\}))-CORR(Y, V\setminus Y).
\end{multline}
Hence, we can see that the correlation function is submodular.

According to \cite{vondrak2007submodularity,krause2014submodular}, it is NP-hard to maximize a submodular function under a matroid constraint. Moreover, it is NP-hard to approximate it within any factor better than $1-1/e$. Therefore, we can conclude that the OTG search problem is NP-hard.

\section{Algorithm 2}
%%%%%%%%%%%%%%%%%%%%%%%%%PUt in full version%%%%%%%%%%%%%%%%%%

\begin{algorithm}
\SetAlgoLined
     \SetKwInOut{Input}{Input}
     \SetKwInOut{Output}{Output}
     \Input{Weighted join graph $G$, a source vertex set $\mathcal{A_S}$, a target vertex set $\mathcal{A_T}$.}
 \Output{A minimal weighted graph $\mathcal{IG}$, which connects all vertices in $\mathcal{A_S}$ and $\mathcal{A_T}$.}
 Load offline pre-calculated data according to \cite{Gubichev:2010:FAE:1871437.1871503}\;
 Initialize output $\mathcal{IG}=\emptyset$\;
 Initialize common landmark set $\mathcal{M}=V$\;
 Initialize minimum weight $MW=\infty$\;
 \For{each vertex $v\in\mathcal{A_S}\cup\mathcal{A_T}$}{
 	Fetch landmark set $M_{v}$ from offline data\;
 	$\mathcal{M}=\mathcal{M}\cap M_{v}$\;
 }
 \For{each common landmark $v_m\in\mathcal{M}$}{
 	$G'=\emptyset$\;
 	\For{each vertex $v\in\mathcal{A_S}\cup\mathcal{A_T}$}{
    	Fetch shortest path $path(v_m,v)$ from offline data\;
        Add $path(v_m,v)$ to $G'$\;
    }
    \eIf{$\mathcal{IG}=\emptyset$ \textbf{or} $G'$ has smaller weight than all graphs in $\mathcal{IG}$}{
        $\mathcal{IG}$:= \{$G'$\};}
    {
    \If{The weight of $G'$ is smaller than $MW$}
  {$\mathcal{IG}=G'$\;
  Set $MW$ the weight of $G'$\;
  }  
  }
 }
Return $\mathcal{IG}$; 
\caption{\label{alg:sp}FindMinG\_ILayer(): find the minimal weighted graphs at the I-layer}
\end{algorithm}

\section{More Experiment Results}
We measure the time performance with regard to various budget ratios on TPC-H dataset. We compare the time performance of our heuristic algorithm with the two optimal methods on TPC-H dataset. We vary the budget ratio from 0.07 to 0.13, where 0.07 and 0.13 were calculated by following the same rationale as in Figure \ref{fig:timeperformance-numinstance-e} (c). We report the results in Figure \ref{fig:timeperformance-budget-h}. 
The main observation is that our heuristic algorithm is much more efficient than both LP and GP for all budget ratios. The advantage of our heuristic algorithm gets larger when the budget ratio grows. 
Second, we observe that, with the growth of budget ratio, our heuristic algorithm takes more time. The reason is straightforward: with more AS-graphs in the I-graph as being affordable, \system needs to spend more time to search through these AS-graphs. 
Similarly, LP and GP consumes more time when the budget ratio is larger, since there are more affordable I-graphs in the search space. 

\begin{figure*}[!hbtp]
\centering
\begin{tabular}{ccc}
	\includegraphics[width=0.33\textwidth]{./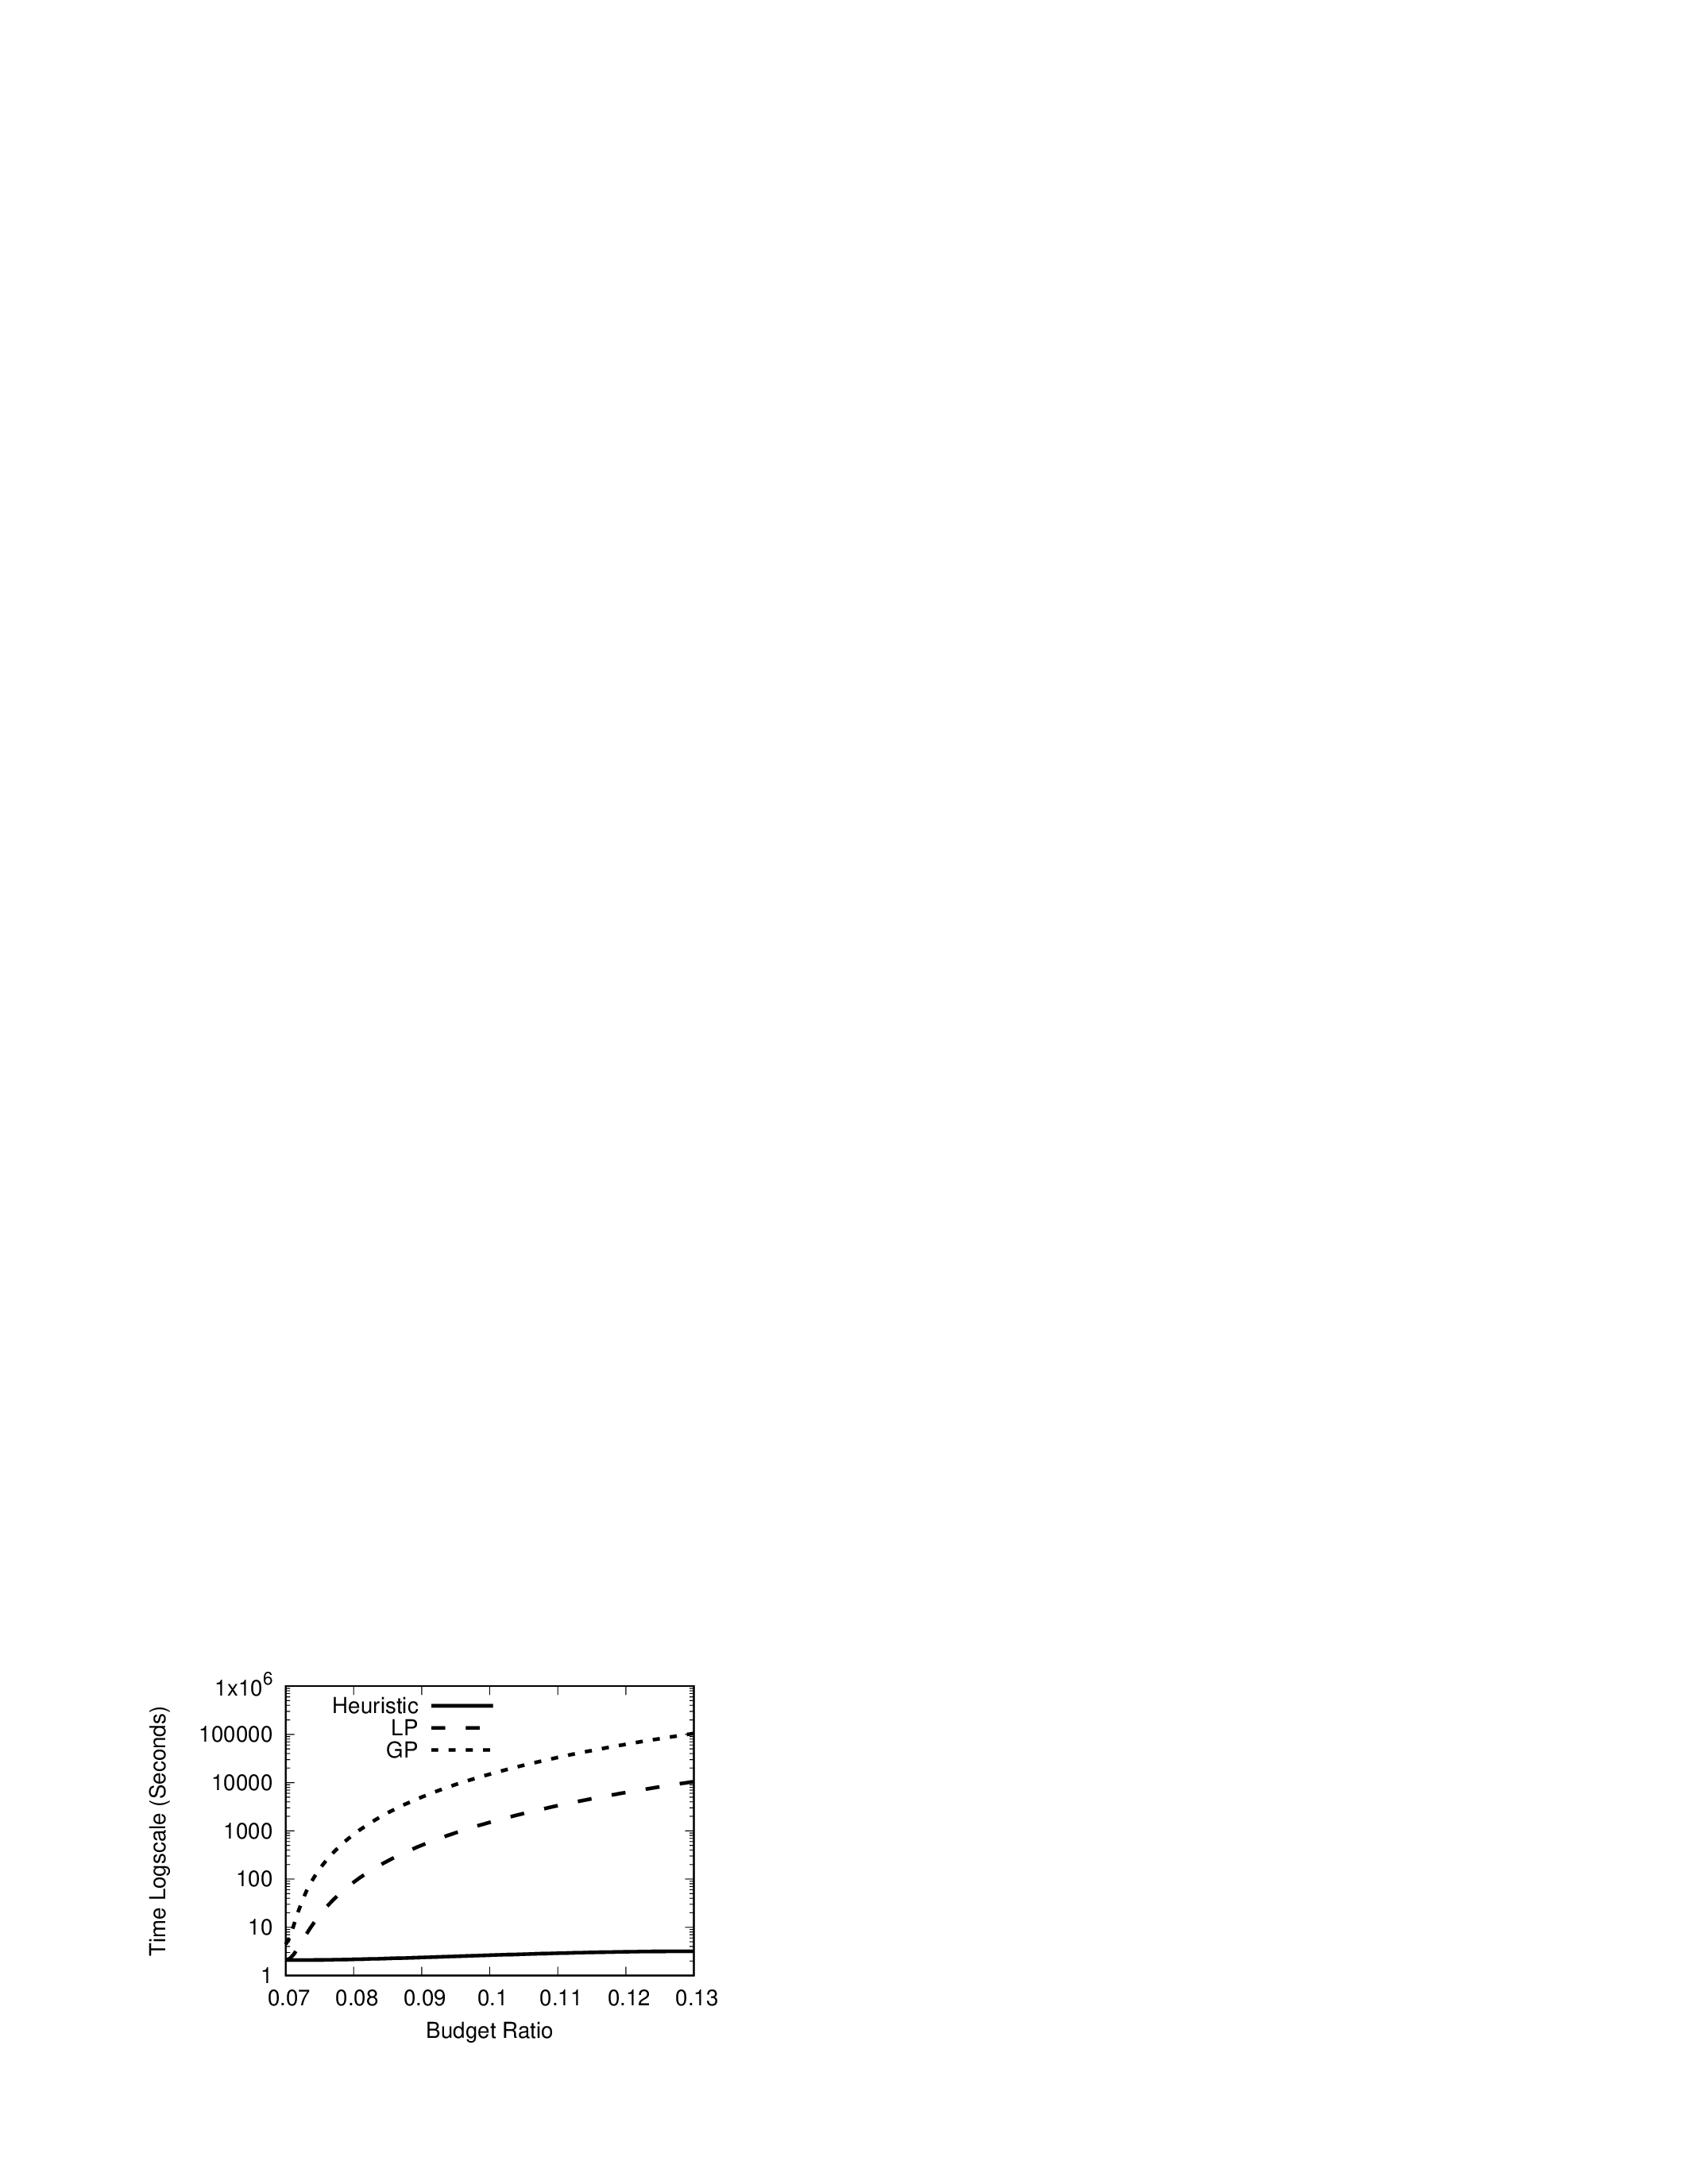}
    &
    \includegraphics[width=0.33\textwidth]{./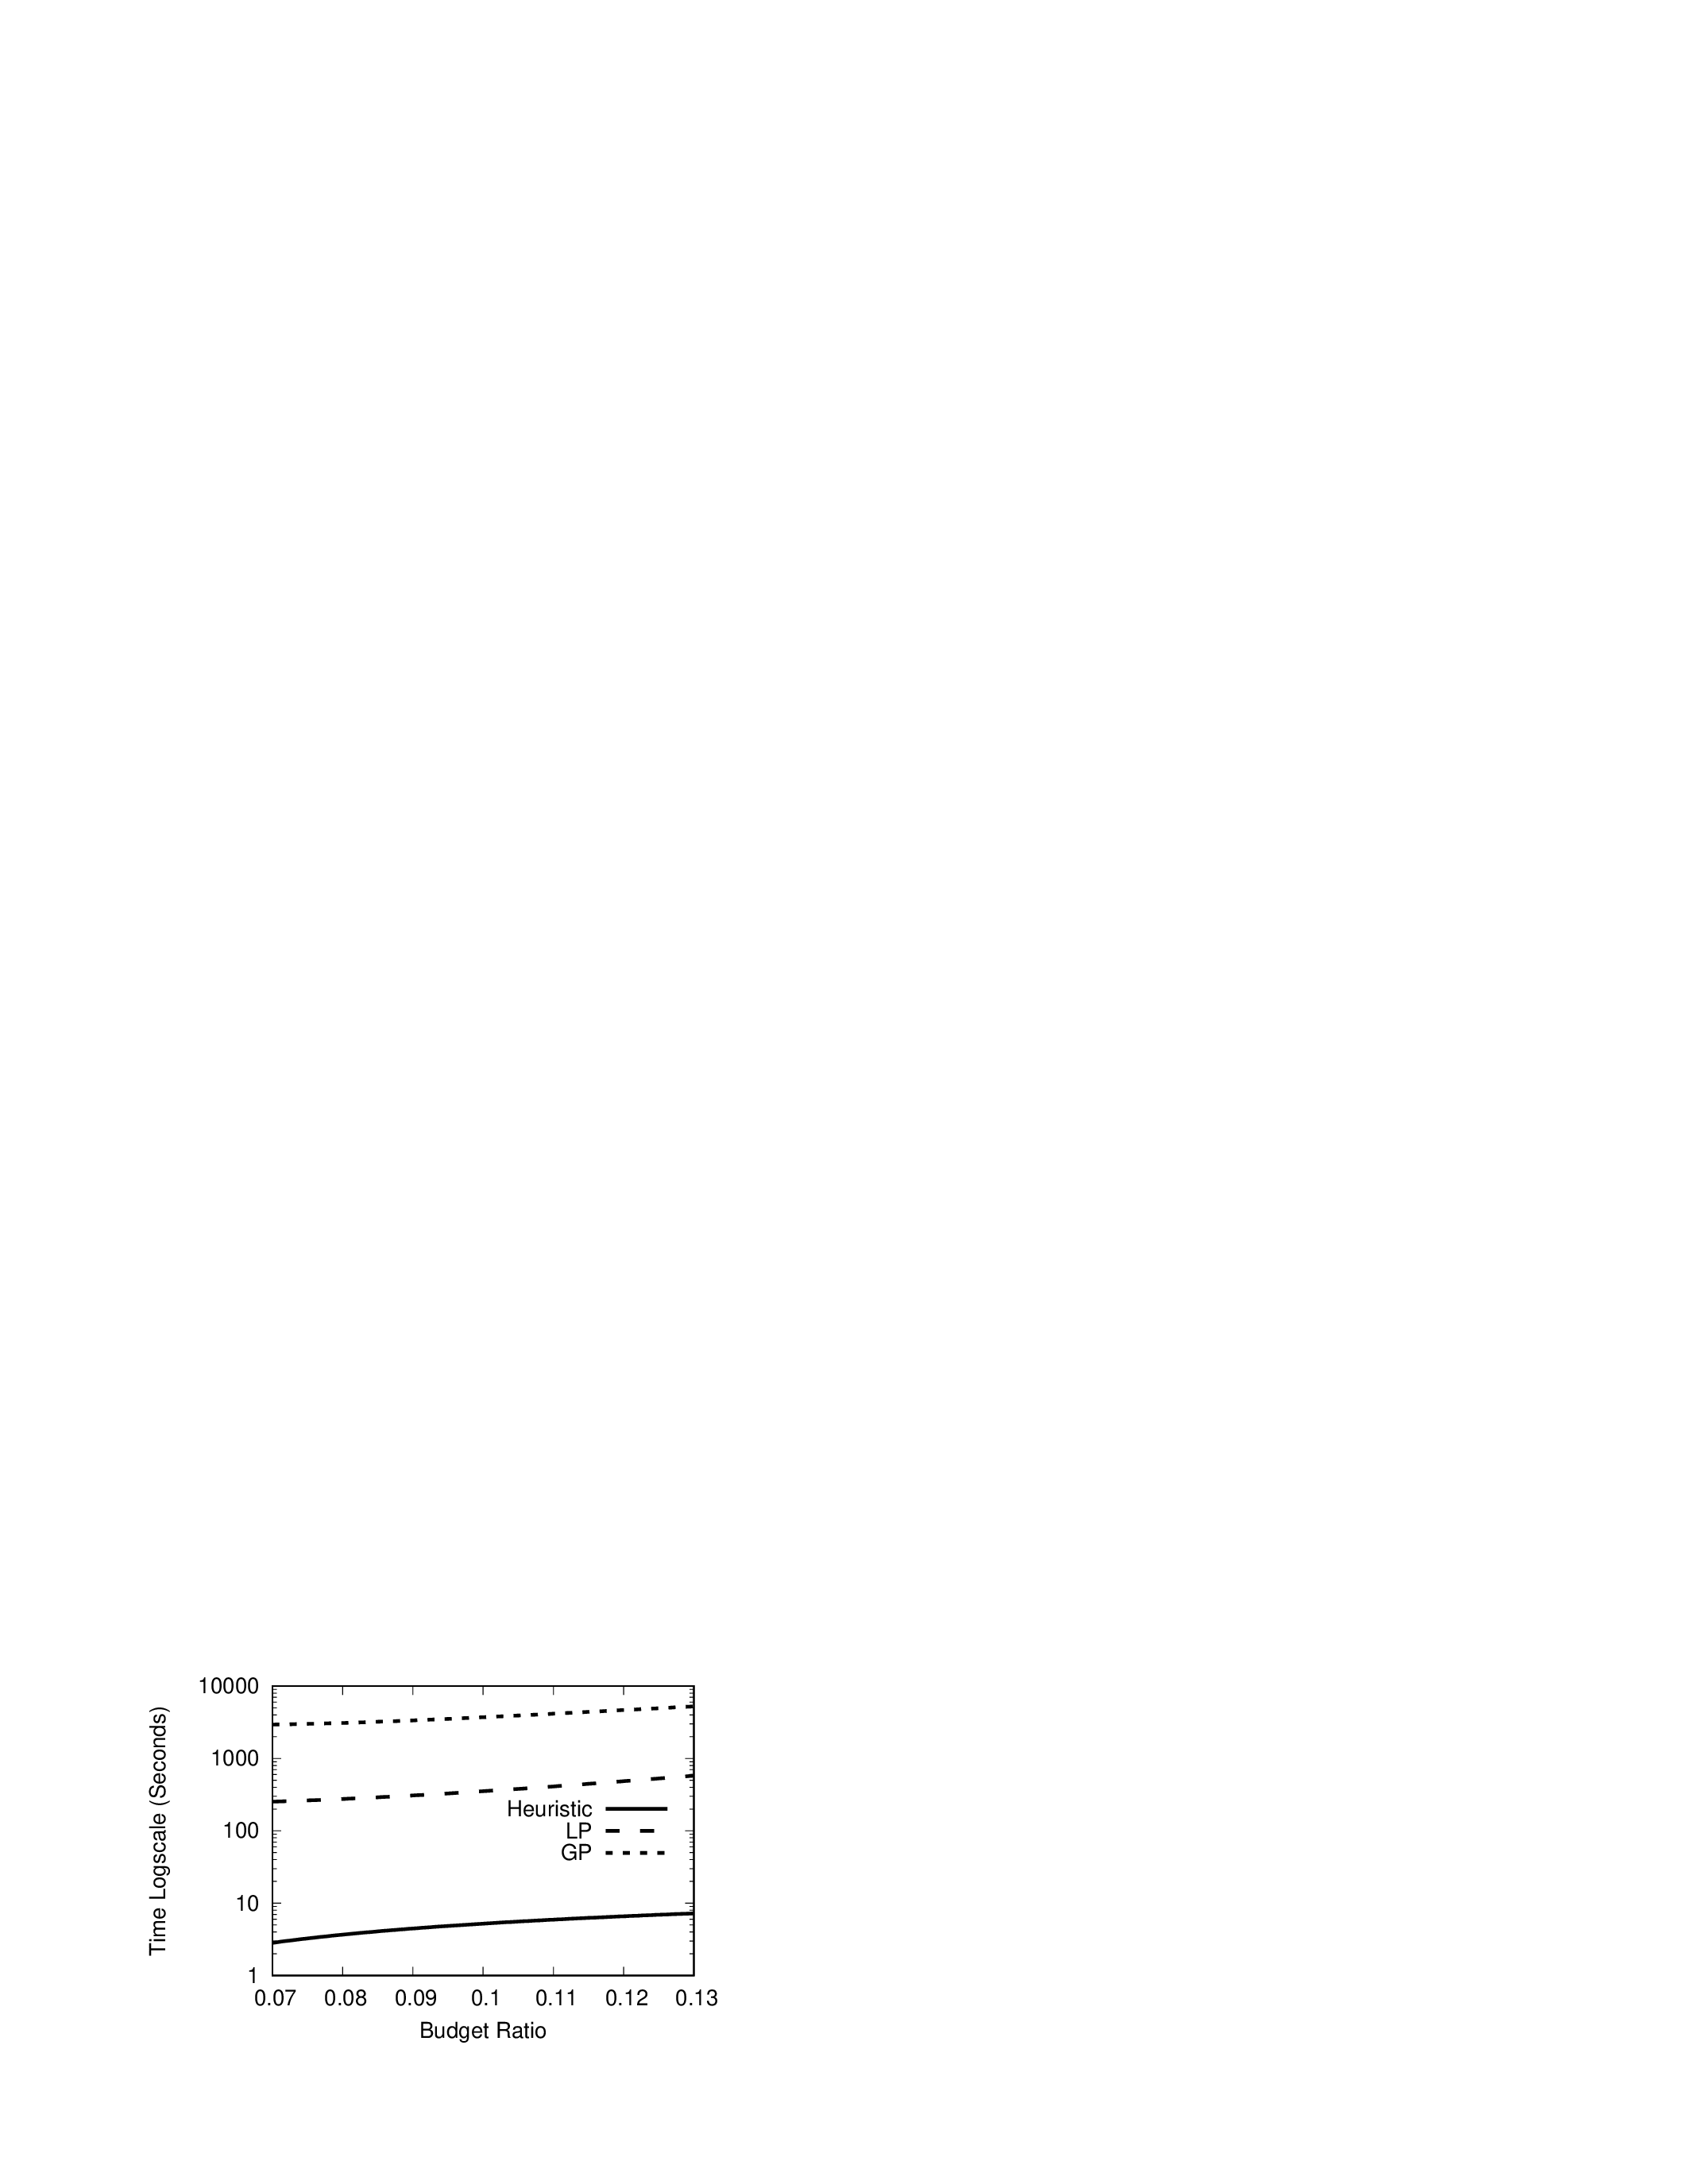}
    &
     \includegraphics[width=0.33\textwidth]{./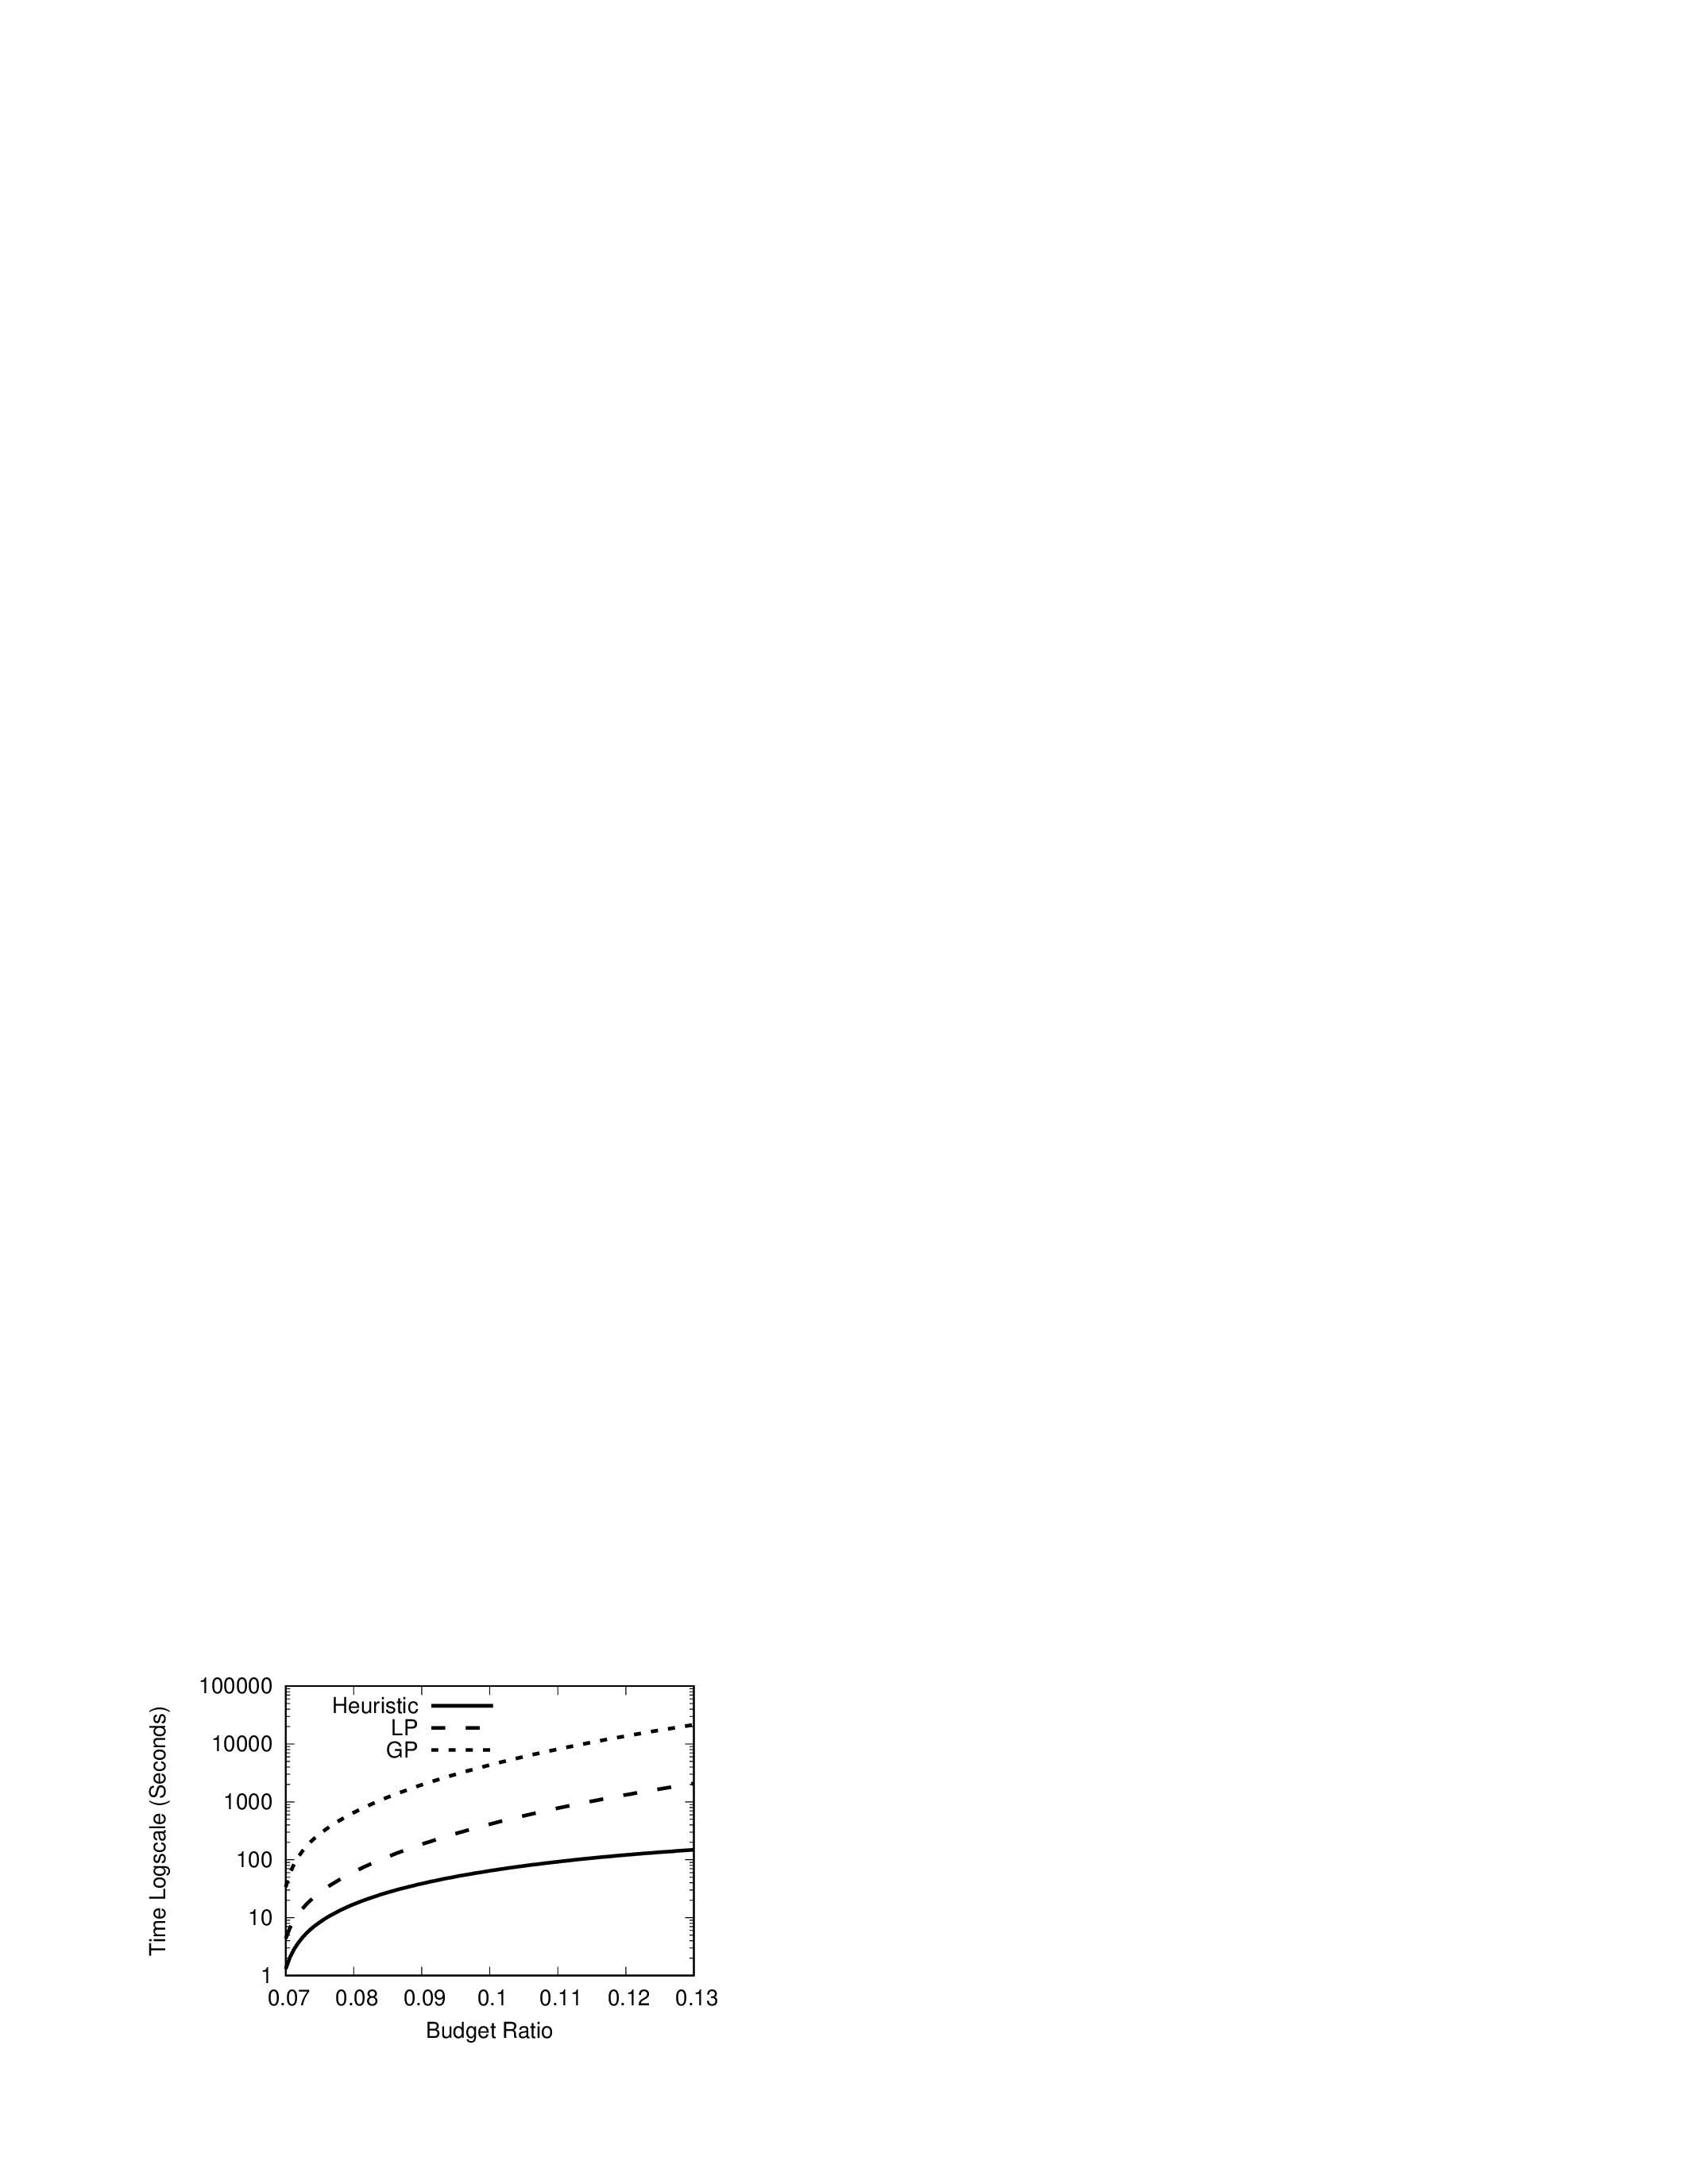}
    \\
    {\small (a) $Q_1$}
    &
    {\small (b) $Q_2$}
    &
    {\small (c) $Q_3$}
\end{tabular}
\caption{\small \label{fig:timeperformance-budget-h} Time Performance w.r.t. various budgets (TPC-H dataset)} 
\vspace{-.55in}
\end{figure*}

\nop{
\begin{algorithm}
\SetAlgoLined  
\SetKwInOut{Input}{Input}
\SetKwInOut{Output}{Output}
\Input{A set of join-able dataframes $tables$, source attribute $S$, target attribute $T$}
\Output{estimated H(S|T)}
\% join attributes\;
Js = Array[String](tables.length - 1)\;
\% intra-table frequency relationship\;
intraf = Array[Double](tables.length)\;
\% inter-table frequency relationship\;
interf = Array[Double](tables.length - 1)\;
\% frequencies of join attributes\;
maps = Array[Map[Row, Long]]((tables.length - 1) * 2)\;
\% average frequency of each join value\;
avgFs = Array[Int]((tables.length - 1) * 2)\;
\For{ i = 0 to tables.length - 2 } {
	Js(i) = tables(i).atts.intersection(tables(i+1).atts)\;
}
\For{ i = 0 to tables.length - 1 } {
	intraf(i) = $p(att1|att2)$\;
}
\For{ i = 0 to Js.length - 1 } {
	maps(i*2) = tables(i).select(Js(i)).countByValue()\;
    maps(i*2 + 1) = tables(i + 1).select(Js(i)).countByValue()\;
}
\For{ i = 0 to maps.length - 1 } {
	\% it should be the average frequency of join-able keys\;
	avgFs(i) = average(maps(i).value)\;
}
\For{ i = 0 to tables.length - 2 } {
	interf(i) = maps(i*2).keys.intersect(maps(i*2+1).keys).size / maps(i*2).keys.size\;
}
\% average frequency of each (T,S) pair\;
F(ST) = 1\;
\For{ avgF in avgFs } {
	F(ST) = F(ST) * avgF\;
}
%\For{ p in interf } {
%	F(ST) = F(ST) * p\;
%}
\For{ p in intraf } {
	F(ST) = F(ST) * p\;
}
d(S) = domain size of S\;
d(T) = domain size of T\;
\% discount, for those non-join-able values
discount = 1\;
\For{ p in interf } {
	discount = discount * p\;
}
\% in total, there are d(S) * d(T) * discount unique (S,T) pairs, each of them has an average frequency of F(ST)\;
estimated join result size: d(S) * d(T) * discount * F(ST)\;
estimated P(S, T) = 1/(d(S)*d(T)*discount)\;
estimated P(T) = 1/d(S)*discount\;
estimated P(S) = 1/d(T)*discount\;
estimated $H(S|T)$ = sum(P(S, T) * log(P(T) / P(S, T)) )\;
$H(S|T)$ = F(ST) * log(d(T))\;
estimated H(S) = d(S) * F(ST) * log(d(T)*discount)\;
Return $H(S) - H(S|T)$\;
%\end{minipage}%
\caption{correlation estimation}
\end{algorithm}
}
